# Supplementary material for: Parameterized Model Checking of Token-Passing Systems
Source: arXiv:1311.4425 source file (2013-11-25)
Supplement: Supplementary file 1 [file oldappendix.tex]

\newpage
\appendix

\blackout{
\section{contributions + intro, old}

\subsubsection{Prenex indexed temporal logic}
\paragraph{Uni-directional ring topology and $\piCTLstarmX$.}
The starting point for our investigation is the cornerstone paper of Emerson and Namjoshi\cite{EN95} that deals with uni-directional rings with one single-valued token.

They provide cutoffs for certain classes of prenex $\CTLstar$ formulas with small number of quantifiers. A {\em cutoff} for a class $C$ of formulas is a constant $c$ such that for every process $P$, every $\phi \in C$, and every $n \in \mathbb{N}$,  $P^n \models \phi$ if and only if $P^c \models \phi$.

%, and additional properties.\footnote{additional properties such as?} 
They state that their proof method can be used to obtain cutoffs for other classes,
but do not give details. We complete the picture by {\bf providing cutoffs}\ak{(RB):where?} 
for prenex $\CTLstar$ formulas with $k$ quantifiers.
%formulas with arbitrary alternations between universal and existential
%quantifiers, of any of the flavours\footnote{what flavours?} defined by Emerson and
%Namjoshi.

\paragraph{Arbitrary topology and $\piLTLmX$.}
Clarke et al.~\cite{CTTV04} built on the ideas of \cite{EN95} to deal with arbitrary parameterized graphs instead of only uni-directional rings.  They provide a decomposition of the PMCP with specifications from $\piLTLmX$ into finitely many finite model-checking problems. However, their result is not constructive and it is not known in general how to find a proper\footnote{What is a proper decomposition?} decomposition\ak{(RB): what is decomposition?} for a
given parameterized graph. 
% {\bf We extend their results}\ak{(RB):where?} by
% giving a decision procedure for infinite collection of graphs that includes common topologies, i.e., cliques, stars, bi-directional rings.\footnote{We give concrete decompositions for bidirectional rings and
%   grids as well as ideas for other graphs.} 
  \sr{We should explain the relationship between decomposition and cutoff.}
  
  \sr{We should try separate those graphs for which $\piCTLstarmX$ is decidable from those for which only $\piLTLmX$ is decidable.}
  \sr{We should prove PMCP for $\piCTLstarmX$ is decidable for all $\pgraph$ that are 
   'homogeneous' in some sense.}
  \sr{We should try to prove that PMCP is un/decidable for $\piCTLstarmX$.}

% \paragraph{Arbitrary topology and multiple tokens.}
% Additionally, we consider the problem of several single-valued tokens
% in rings and arbitrary graphs. {\bf We show} that the PMCP remains
% \emph{decidable} in many cases, and moreover, that existing cutoff and
% decomposition results still hold(?). However, in case the tokens can be
% distinguished, we show that PMCP is \emph{undecidable}. 

\paragraph{Arbitrary topology and direction-aware tokens.}
For unidirectional rings with a multi-valued token, undecidability has
been shown by Suzuki~\cite{Suzuki}, and for a binary token by
Emerson and Namjoshi~\cite{EN95}. Emerson and Kahlon~\cite{EK04} have shown that
decidability is preserved if there is a fixed bound on the number of
changes to the token value in any execution of the system, and
that this holds even in bidirectional rings where processes can
choose in which direction to send the token, but cannot detect from
which direction tokens are received. This inspired four flavors of direction-aware systems 
depending on 
a) whether they know from whom they receive the token,
b) whether processes can choose\ak{(RB): clarify sense/control notations} 
to whom they send it. 
We write Y/Y for the case that the answer to both questions is ``Yes'', 
write N/Y if the answer to a) is ``No'' and b) is ``Yes'', etc.
In this paper we study all four variations.
~\cite{CTTV04} show that  PMCP is decidable for the N/N case 
and~\cite{EK04} show that PMCP is decidable for the N/Y case on bi-directional rings
\ak{1-indexed? do they have bounds on the number of changes of the \emph{direction}?}. 
In contrast\ak{(RB) to what?}, we show that PMCP is undecidable for Y/Y on bi-directional rings 
(but decidable if the number of direction changes is bounded), 
undecidable for N/Y for certain graphs, 
and decidable for the Y/N case.

\subsubsection{Atom-quantified temporal logic}
We show that allowing quantification over Boolean combinations of atoms is quite expressive. 
For instance, over rings (and certain other topologies) one can express 
that the number of vertices in the topology is divisible by $2$ 
(or any other congruence relation).

It is known [Igor] that PMCP is undecidable for AQLTL[F,G] even with no communication. 
We provide a fragment of AQLTL[F,G] for which PMCP over rings is decidable. 
We show that AQCTL is undecidable over ...

\subsubsection{Prenex indexed temporal logic}

A popular specification language for parameterized systems is indexed temporal logic (ITL).\note[SR]{can anyone justify this sentence? o/w it should be weakened.} The main attribute of this language is that atomic propositions are indexed by processes --- thus $p_i$ is an atom that means that process $i$ satisfies atomic proposition $p$. Fix a temporal logic \TL\ such as \CTLstarmX. The syntax of ITL is like TL except that one allows quantifiers such as $\exists i \phi$ which mean `there is a process satisfying $\phi$'. Since processes are modeled as LTSs, the semantics of ITL is defined over the parallel compositions of LTSs. There are a number of popular fragments of ITL. For integer $k$ write $\kTL$ for the formulas of the form $Q_1 x_1 \cdots Q_k x_k \, \phi$ where $\phi$ is a \TL\ formula (over indexed propositions). {\em Prenex indexed temporal logic (PITL)}, written $\piTL$, is defined as the union $\cup_k \kTL$.

\paragraph{Uni-directional ring topology and $\piCTLstarmX$.}
The starting point for our investigation is the cornerstone paper of Emerson and Namjoshi\cite{EN95} that deals with uni-directional rings with one single-valued token.

They provide cutoffs for certain classes of prenex $\CTLstar$ formulas with small number of quantifiers. A {\em cutoff} for a class $C$ of formulas is a constant $c$ such that for every process $P$, every $\phi \in C$, and every $n \in \mathbb{N}$,  $P^n \models \phi$ if and only if $P^c \models \phi$.

%, and additional properties.\footnote{additional properties such as?} 
They state that their proof method can be used to obtain cutoffs for other classes,
but do not give details. We complete the picture by {\bf providing cutoffs}\ak{(RB):where?} 
for prenex $\CTLstar$ formulas with $k$ quantifiers.
%formulas with arbitrary alternations between universal and existential
%quantifiers, of any of the flavours\footnote{what flavours?} defined by Emerson and
%Namjoshi.

\paragraph{Arbitrary topology and $\piLTLmX$.}
Clarke et al.~\cite{CTTV04} built on the ideas of \cite{EN95} to deal with arbitrary parameterized graphs instead of only uni-directional rings.  They provide a decomposition of the PMCP with specifications from $\piLTLmX$ into finitely many finite model-checking problems. However, their result is not constructive and it is not known in general how to find a proper\footnote{What is a proper decomposition?} decomposition\ak{(RB): what is decomposition?} for a
given parameterized graph. {\bf We extend their results}\ak{(RB):where?} by
giving a decision procedure for infinite collection of graphs that includes common topologies, i.e., cliques, stars, bi-directional rings.\footnote{We give concrete decompositions for bidirectional rings and
  grids as well as ideas for other graphs.} 
  \sr{We should explain the relationship between decomposition and cutoff.}
  
  \sr{We should try separate those graphs for which $\piCTLstarmX$ is decidable from those for which only $\piLTLmX$ is decidable.}
  \sr{We should prove PMCP for $\piCTLstarmX$ is decidable for all $\pgraph$ that are 
   'homogeneous' in some sense.}
  \sr{We should try to prove that PMCP is un/decidable for $\piCTLstarmX$.}

% \paragraph{Arbitrary topology and multiple tokens.}
% Additionally, we consider the problem of several single-valued tokens
% in rings and arbitrary graphs. {\bf We show} that the PMCP remains
% \emph{decidable} in many cases, and moreover, that existing cutoff and
% decomposition results still hold(?). However, in case the tokens can be
% distinguished, we show that PMCP is \emph{undecidable}. 

\paragraph{Arbitrary topology and direction-aware tokens.}
For unidirectional rings with a multi-valued token, undecidability has
been shown by Suzuki~\cite{Suzuki}, and for a binary token by
Emerson and Namjoshi~\cite{EN95}. Emerson and Kahlon~\cite{EK04} have shown that
decidability is preserved if there is a fixed bound on the number of
changes to the token value in any execution of the system, and
that this holds even in bidirectional rings where processes can
choose in which direction to send the token, but cannot detect from
which direction tokens are received. This inspired four flavors of direction-aware systems 
depending on 
a) whether they know from whom they receive the token,
b) whether processes can choose\ak{(RB): clarify sense/control notations} 
to whom they send it. 
We write Y/Y for the case that the answer to both questions is ``Yes'', 
write N/Y if the answer to a) is ``No'' and b) is ``Yes'', etc.
In this paper we study all four variations.
~\cite{CTTV04} show that  PMCP is decidable for the N/N case 
and~\cite{EK04} show that PMCP is decidable for the N/Y case on bi-directional rings
\ak{1-indexed? do they have bounds on the number of changes of the \emph{direction}?}. 
In contrast\ak{(RB) to what?}, we show that PMCP is undecidable for Y/Y on bi-directional rings 
(but decidable if the number of direction changes is bounded), 
undecidable for N/Y for certain graphs, 
and decidable for the Y/N case.

{\color{black!50}
\begin{question}
Is there $\pgraph$ such that $\PMCP$ is undecidable for \kCTLstarmX?
\end{question}
}

\subsubsection{Atom-quantified temporal logic}
We show that allowing quantification over Boolean combinations of atoms is quite expressive. 
For instance, over rings (and certain other topologies) one can express 
that the number of vertices in the topology is divisible by $2$ 
(or any other congruence relation).

It is known [Igor] that PMCP is undecidable for AQLTL[F,G] even with no communication. 
We provide a fragment of AQLTL[F,G] for which PMCP over rings is decidable. 
We show that AQCTL is undecidable over ..

\section{Direction-Aware}

One can define direction-awareness so that for each element of $\{\tsnd,\trcv\}$ there are three possible modes. For instance, for $\trcv$ (and similarly for $\tsnd$) a process may satisfy 
\begin{enumerate}
\item[$N$] for all states without the token the process does not know from which in-direction it receives.
\item[$K$] for all states without the token the process may know, but not block, from which in-direction the token was received. 
\item[$C$] for all states without the token may know, and may block, from which in-direction the token was received.
\end{enumerate}

Let $N$ mean 'not know', $K$ mean 'know' and $C$ mean 'can choose'.
For $\trcv$, mode $C$ is defined as in Section~\ref{sec:DATPS}, $N$ is defined by having $|dir_{\trcv}| = 1$, and $K$ is defined by restricting the process to always be able to receive the token no matter what in-direction is used (although it may change state according to the in-direction).

Looking at the definitions note that $C$ implies $K$, which itself implies $N$. 

Thus there are nine possible modes, each one designated by an element of the set $\{N,K,C\}^2$ 
The first component refers to the mode of $\trcv$, and the second to the mode of $\tsnd$.
The following results are for prenex indexed \LTLmX. Note the surprising (at first) asymmetry between $(N,K)$ and $(K,N)$.

\begin{theorem}
PMCP is decidable for $(K,N)$ and $(N,N)$, and undecidable for all the other 8 modes.
\end{theorem}

\begin{proof}
\begin{enumerate}
\item $(K,N)$ decidable follows from a slight extension of CTTV; thus $(N,N)$ is also decidable.
\item $(C,N)$ is undecidable using a proof similar to that in proposition~\ref{prop:NC}.
\item $(N,K)$ is undecidable using a proof similar to that in proposition~\ref{prop:NC}; thus the following are also undecidable: $(N,C)$, $(K,K)$, $(C,K)$, $(K,C)$ and $(C,C)$.
\end{enumerate}
\end{proof}

\section{Simple TPSs}

We aim to address the following problems:
\begin{problem}
Are there any undecidability results in $\PMCP$ for TPSs with single value-less token?
\end{problem}

\begin{answer}
No, but we will give the first one: for bidirectional rings with
direction-awareness.
\end{answer}

\begin{answer}
Also, ITL (and the fragment QATL) on rings has undecidable PMCP.
\end{answer}

\begin{question}
Compare cutoff/decidability proofs of CTTV, EN, GS92 (TPS can be expressed in terms of PR).
Exactly what types of cutoffs/decompositions hold in all cases? Rings,Graphs and $\piLTLmX$,$\piCTLstarmX$?
\end{question}

\subsubsection{Prenex ITL}

\begin{question}
What fragment of ITL has cutoffs?
%Let $\Pspec_k$ be the formulas of QATL the nesting depth of temporal operators is at most $k$. Then the second results says any constant cutoff for $\Pspec_k$ is at least $k$. Does $\Pspec_k$ have constant cutoff?
\end{question}

\section{Musings} 

\begin{enumerate}
\item If processes know the sender but not the recipient then $\PMCP$ is decidable (the CTTV abstraction works).? 

\item If processes know the recipient but not the sender it is decidable for
bidirectional rings and 1-indexed specifications, otherwise we don't know.

\item There is a cutoff for finitely many identical unary-tokens (this generalises EK04 and CTTV04).
What about binary-token with bounded number of value changes?

\item What about binary-token with finitely many (but unknown number) of value changes?  

\item Push Suz/EK to graphs.

\item EFM99 show that liveness (over actions) for broadcast protocols is undecidable. 
The proof uses about 6 different broadcast actions. What if we restrict to a single action? 

\item What happens to the results of EFM99, EmersonK03c, EN98, VASS, if instead of AP = Actions, we look at $k$-index?

\item Look at EK03 and see what happends to results if we remove the controller process $C$. Do the results change? Cf. GS92.

\item What about systems (BiRings or general graphs with outdegree $>1$)
  which are not direction-aware, but have binary token? (decidable?)

\item What about systems (BiRings or general graphs) with multiple
  indistinguishable tokens, which may start in different processes?
  (i.e. no leader process exists or can be elected; decidable?)

\item Can we obtain decidability results for classes of graphs and
  specifications by looking at network grammars? I.e., can we find a
  connection between network grammars and suitable reductions \`a la
  CTTV? 

\item What happen with undecidability results (binary tokens for example)
  if the initial configuration doesn't allow processes to choose a leader?

\section{Multi-valued TPSs for $\piLTLmX$}

TPSs can be modeled with PR. The latter has decidable $\PMCP$ over
cliques/stars using monotonicity arguments (ala GS92).

\begin{theorem}[GS92]
$\PMCP$ with pairwise rendezvous for cliques and  $1$-indexed $\omega$-regular specs is decidable.
\end{theorem}

\begin{question}
For which $\pgraph,\pspec$ is $\PMCP(\pgraph,\pspec,PR)$ decidable?
\end{question}

\begin{proposition}
$\PMCP$ is decidable for multi-valued TPS (on arbitrary graphs we have $\piLTLmX$, on rings we have $\piCTLstarmX$) if we restrict to systems in which from every state $q$ with the token and every value $v$ there is a path from $q$ in which the first time it sends the token it is with value $v$.
\end{proposition}

\end{enumerate}
}
